# Supplementary material for: Generalized Paxos Made Byzantine (and Less Complex)
Source: arXiv:1708.07575 source file (2017-10-19)
Supplement: Supplementary file 1 [file appendix.tex]

\section{Crash-fault Tolerant Protocol}
\label{app:cft}
\textbf{Simplified Problem} Generalized Paxos solves the problem of agreeing on increasing sets of values. These sets of commands are defined to be \textit{c-structs}, which are structures more generic than sequences since they allow for command sequences $\sigma$ and $\tau$ to be equivalent despite having different contents. This is possible because there is a custom \textit{equivalence relation} between \textit{c-structs}. However, this generalization comes at the cost of increased complexity. To present a simpler version of the protocol, our simplification does away with the generic equivalence relation and defines it to be as the equivalence relation between command histories.  \par
\textbf{Protocol} \textcolor{red}{Finish CFT protocol description}
\begin{table}[h!]
	
	\centering
	\begin{tabular}{ |c|c|}
		\hline
		\multicolumn{2}{|c|}{Notation}\\
		\hline
		Symbol & Definition \\
		\hline
		$\sqcup$ & least upper bound \\
		\hline
		$\sqcap$ & greatest lower bound \\
		\hline
		$\bullet$ & append operator \\
		\hline
	\end{tabular} 
	\caption{Notation for the pseudocode} 
	\label{table:1}
\end{table}

\begin{algorithm}
	\caption{Generalized Paxos - Proposer p}
	\begin{algorithmic}[1]
		
		\Function{propose}{\textit{C}}
		\If{fast\_ballot}
		\State \Call{send}{$fast, C$} to Acceptors;
		\Else
		\State \Call{send}{\textit{propose, C}} to Leader;
		\EndIf
		\EndFunction

	\end{algorithmic}
\end{algorithm}

\begin{algorithm}
	\caption{Generalized Paxos - Leader l}
	\textbf{Local variables:} $ballot_l = 0,\ maxTried_l = \bot,\ C_l = \bot, messages = \bot$
	\begin{algorithmic}[1]
		\State \textbf{upon} \textit{receive(propose, C)} from proposer $p_i$ \textbf{do} 
		\State \hspace{\algorithmicindent} $C_l = C$;
		\State \hspace{\algorithmicindent} \Call{phase\_1a}{$ $};
		\State
		\State \textbf{upon} \textit{receive(statement)} from acceptor $a_i$ \textbf{do}
		\State \hspace{\algorithmicindent}  $messages[ballot_l][a_i] = statement$;
		\State \hspace{\algorithmicindent} \textbf{if} $\#(messages) \geq \lfloor \frac{N}{2} \rfloor +1$ \textbf{then} 
		\State \hspace{\algorithmicindent}\hspace{\algorithmicindent} \Call{phase\_2a}{$ballot_l, Q$};
		\State
		%\item[] % unnumbered empty line
		\Function{phase\_1a}{}
		\State \Call{send}{$p1a, ballot_l$} to Acceptors;
		\EndFunction
		
		\State
		\Function{phase\_2a}{$bal, Q$}
		\State $maxTried_l$ = \Call{proved\_safe}{$Q, bal$};
		\State $maxTried_l = maxTried_l \bullet C_l$;
		\State \Call{send}{$p2a,ballot_l, maxTried_l$} to Acceptors;
		\EndFunction
		
		\State
		\Function{proved\_safe}{$ballot$}
		\State $maxTried = \bot$;
		\State \textbf{for} $val$ in $message[ballot]$ \textbf{do}
		\State \hspace{\algorithmicindent} \textbf{if} $maxTried = \bot$ or $\Call{is\_prefix}{val, maxTried}$ \textbf{then}
		\State\hspace{\algorithmicindent}\hspace{\algorithmicindent} $maxTried = val$;
		\State \textbf{end for}
		\State \textbf{return} $maxTried$;
		\EndFunction
		
			\State
		\Function{is\_prefix}{$new\_sequence, old\_sequence$}
		\If {$\lVert old\_sequence \rVert > \lVert new\_sequence \rVert$}
		\State \textbf{return} \textit{false};
		\EndIf
		
		\State
		\item[] outer:	
		\State \textbf{for} $c_{old}$ in $old\_sequence$ \textbf{do}
		\State \hspace{\algorithmicindent} \textbf{for} $c_{new}$ in $new\_sequence$ \textbf{do}
		\State\hspace{\algorithmicindent}\hspace{\algorithmicindent} \textbf{if} $c_{old} = c_{new}$ \textbf{then}
		\State \hspace{\algorithmicindent}\hspace{\algorithmicindent}\hspace{\algorithmicindent} \textbf{continue} \textit{outer};
		
		\State \hspace{\algorithmicindent}\hspace{\algorithmicindent} \textbf{else if} !\Call{are\_commutative}{$c_{old}, c_{new}$} \textbf{then}
		\State\hspace{\algorithmicindent}\hspace{\algorithmicindent}\hspace{\algorithmicindent} \textbf{return} \textit{false};
		\State \hspace{\algorithmicindent}\textbf{end for}
		\State \hspace{\algorithmicindent}\textbf{return} \textit{false};
		\State \textbf{end for}
		\State
		\State \textbf{return} \textit{true};
		\EndFunction
		
	\end{algorithmic}
\end{algorithm}

\begin{algorithm}
	\caption{Generalized Paxos - Acceptor a}
	\textbf{Local variables: } $bal_a = 0,\ val_a = \bot$ 
	\begin{algorithmic}[1]
		
		\State \textbf{upon} \textit{receive(fast, val)} from proposer \textit{p} \textbf{do}
		\State \hspace{\algorithmicindent} \Call{phase\_2b\_fast}{$val$};
		
		\State
		\State \textbf{upon} \textit{receive(p1a, ballot)} from leader \textit{l} \textbf{do}
		\State \hspace{\algorithmicindent} \Call{phase\_1b}{$ballot, l$};
		
		\State
		\State \textbf{upon} \textit{receive(p2a, ballot, value)} from leader \textit{l} \textbf{do}
		\State \hspace{\algorithmicindent} \Call{phase\_2b\_classic}{$ballot, value$};
		
		\State
		\Function{phase\_1b}{$m, l$}
		\If {$bal_a < m$}
		\State \Call{send}{$p1b, m, bal_a, val_a$} to leader l;
		\State $bal_a = m$;
		\EndIf
		\EndFunction
		
		\State
		\Function{phase\_2b\_classic}{$m, v$}
		\State $k = max(i\ |\ (i < m) \wedge (\exists a \in Q :\ val_a[i]\ \neq null))$;
		\If {$m \geq k$}
		\State $val_a = v$;
		\State \Call{send}{$p2b, bal_a, val_a$} to learners;
		\EndIf
		\EndFunction
		
		\State
		\Function{phase\_2b\_fast}{$v$}
		\State $k = max(i\ |\ (i < m) \wedge (\exists a \in Q :\ val_a[i]\ \neq null))$;
		\If {$bal_a == k$}
		\State $val_a = val_a \bullet v$;
		\State \Call{send}{$p2b, bal_a, val_a$} to learners;
		\EndIf
		\EndFunction
		
	\end{algorithmic}
\end{algorithm}

\begin{algorithm}
	\caption{Generalized Paxos - Learner l}
	\textbf{Local variables: } $learned = \bot, messages = \bot$ 
	\begin{algorithmic}[1]
		\State \textbf{upon} \textit{receive($p2b, bal, val$)} from acceptor $a_i$ \textbf{do}
		\State \hspace{\algorithmicindent} $messages[bal][a_i] = val$;
		\State \hspace{\algorithmicindent} \textbf{if} {($fast\_ballot$ and $\#(messages[bal]) \geq \lceil \frac{3N}{4} \rceil$) or
			\State \hspace{\algorithmicindent} \hspace{\algorithmicindent}	($classic\_ballot$ and $\#(messages[bal]) \geq \lfloor \frac{N}{2}\rfloor+1$)} \textbf{then}
		\State \hspace{\algorithmicindent} \hspace{\algorithmicindent} \hspace{\algorithmicindent} $learned = learned \sqcup val$;
	\end{algorithmic}
\end{algorithm}
